# Supplementary material for: Model Identification Adaptive Control with $\rho$-POMDP Planning
Source: arXiv:2505.09119 source file (2025-05-22)
Supplement: Supplementary file 1 [file 99_00_appendix.tex]

\appendix

% Appendix trick from
% https://ckadapa.wordpress.com/2019/09/24/formatting-equations-in-appendix-in-latex/

% reset the counter
\setcounter{equation}{0}
\setcounter{table}{0}
\setcounter{figure}{0}

\subsection{Proofs from THE KYLE}

When options are feasible when executed under a budget for their decision epoch, \algname\ can maintain feasibility.
To show this, we first define the concept of a locally feasible option in~\cref{def_appendix:locally-feasible-option} below.
Informally, such an option ensures it does not go over a budget set while it is in control.

\begin{definition}
    \label{def_appendix:locally-feasible-option}
    For an option $\hat{a}_\ep$ chosen at decision epoch $e$ in $b_\ep$, given budget $\hat{\mathbf{c}}_\ep$, is \emph{locally feasible} if $\mathbf{Q}_\mathbf{C}^\pi(b_\ep, \hat{a}_\ep) \leq \hat{\mathbf{c}}_e$.
\end{definition}

Two additional types of feasibility, one-step global and global, are stated in Definitions~\ref{def_appendix:one-step-global-feasibility} and~\ref{def_appendix:global-feasibility}, respectively.
Informally, the first describes an option that can be applied once and guarantee it does not go over the allotted budget.

\begin{definition}
    \label{def_appendix:one-step-global-feasibility}
    An option $\hat{a}_\ep$ chosen at decision epoch $\ep$ in $b_\ep$ is \emph{one-step globally feasible} if $\tilde{\mathbf{c}}_{\ep-1} + \mathbf{Q}_{\mathbf{C},\ep}^\pi(b_\ep, \hat{a}_\ep) \leq \hat{\mathbf{c}}$.
\end{definition}

This second definition states that an agent is globally feasible if the original constraints from~\cref{eq:cpomdp-objective-constraints} are satisfied.

\begin{definition}
    \label{def_appendix:global-feasibility}
    An algorithm or policy $\pi$ is said to be \emph{globally feasible} if $\mathbf{V}_{\mathbf{C}}^\pi(b_0) \leq \hat{\mathbf{c}}$.
\end{definition}

With these definitions,~\cref{prop_appen:local-feasible-option-with-hatct-one-step-globally-feasible} below shows that for a CPOSMDP, if a locally feasible option is chosen with a particular assignment of $\hat{\mathbf{c}}_\ep$, then it ensures that one-step is globally feasible.

\begin{proposition}
    \label{prop_appen:local-feasible-option-with-hatct-one-step-globally-feasible}
    For policy $\pi$ and locally feasible option $\hat{a}_\ep$, if $\hat{\mathbf{c}}_\ep$ = $\frac{\hat{\mathbf{c}} - \tilde{\mathbf{c}}_{\ep-1}}{\gamma^{t_{\ep-1}}} \geq 0$ with $\tilde{\mathbf{c}}_0 = \mathbf{0}$ at decision epoch $\ep$, which is at time $t_{\ep-1}$ and accumulated costs $\tilde{c}_{\ep-1}$, then $\hat{a}_\ep$ is one-step globally feasible.
\end{proposition}

\begin{proof}
By definition of a locally feasible option and the choice of $\hat{\mathbf{c}}_e$:
\begin{align*}
    &\mathbf{Q}_{\mathbf{C}}(b_\ep, \hat{a}_\ep) \leq \hat{\mathbf{c}}_\ep \\
    &\mathbb{E}\Big[\sum_{i=0}^\infty \gamma^i \mathbf{C}(b_i', a_i') | b_0' {=} b_\ep, a_0' {=} \hat{a}_\ep, \pi \Big] \leq \hat{\mathbf{c}}_\ep \\
    &\mathbb{E}\Big[\sum_{j=t_{\ep-1}}^\infty \gamma^{i-t_{\ep-1}} \mathbf{C}(b_j, a_j) | b_{t_{\ep-1}} {=} b_\ep, a_{t_{\ep-1}} {=} \hat{a}_\ep, \pi \Big] \leq \hat{\mathbf{c}}_\ep \\
    %&\mathbb{E}\Big[\sum_{j=t_{\ep-1}}^\infty \gamma^{i-t_{\ep-1}} \mathbf{C}(b_j, a_j) | b_{t_{\ep-1}} = b_\ep, a_{t_{\ep-1}} = \hat{a}_\ep, \pi \Big] \leq \frac{\hat{\mathbf{c}} - \tilde{\mathbf{c}}_{\ep-1}}{\gamma^{t_{\ep-1}}} \\
    &\mathbb{E}\Big[\sum_{j=t_{\ep-1}}^\infty \gamma^{i-t_{\ep-1}} \mathbf{C}(b_j, a_j) | \text{---} \Big] \leq \frac{\hat{\mathbf{c}} - \tilde{\mathbf{c}}_{\ep-1}}{\gamma^{t_{\ep-1}}} \\
    %&\tilde{\mathbf{c}}_{\ep-1} + \gamma^{t_{\ep-1}} \mathbb{E}\Big[\sum_{j=t_{\ep-1}}^\infty \gamma^{i-t_{\ep-1}} \mathbf{C}(b_j, a_j) | b_{t_{\ep-1}} = b_\ep, a_{t_{\ep-1}} = \hat{a}_\ep, \pi \Big] \leq \hat{\mathbf{c}} \\
    &\tilde{\mathbf{c}}_{\ep-1} + \gamma^{t_{\ep-1}} \mathbb{E}\Big[\sum_{j=t_{\ep-1}}^\infty \gamma^{i-t_{\ep-1}} \mathbf{C}(b_j, a_j) | \text{---} \Big] \leq \hat{\mathbf{c}} \\
    %&\tilde{\mathbf{c}}_{\ep-1} + \mathbb{E}\Big[\sum_{j=t_{\ep-1}}^\infty \gamma^{i} \mathbf{C}(b_j, a_j) | b_{t_{\ep-1}} = b_\ep, a_{t_{\ep-1}} = \hat{a}_\ep, \pi \Big] \leq \hat{\mathbf{c}} \\
    &\tilde{\mathbf{c}}_{\ep-1} + \mathbb{E}\Big[\sum_{j=t_{\ep-1}}^\infty \gamma^{i} \mathbf{C}(b_j, a_j) | \text{---} \Big] \leq \hat{\mathbf{c}} \\
    &\tilde{\mathbf{c}}_{\ep-1} + \mathbf{Q}_{\mathbf{C},t}^\pi(b_\ep, \hat{a}_\ep) \leq \hat{\mathbf{c}} \text{.}
\end{align*}
Thus, by~\cref{def_appendix:one-step-global-feasibility}, $\hat{a}_e$ is one-step globally feasible.
\end{proof}

Combining these results yields that \algname\ is globally feasible when its options are one-step globally feasible.

\begin{proposition}
    \label{prop_appen:cobets-globally-feasible}
    \algname\ is globally feasible if all its options $\hat{a}_e$ are locally feasible given \algname\ dynamic assignments of $\hat{\mathbf{c}}_\ep \geq 0$ for all $\ep$.
\end{proposition}

\begin{proof}
By construction.
Consider any decision epoch $\ep$.
As given, consider any \algname\ option $\hat{a}_\ep$.
By definition of \algname, it assigns $\hat{\mathbf{c}}_\ep = \frac{\hat{\mathbf{c}} - \tilde{\mathbf{c}}_{\ep-1}}{\gamma^{t_{\ep-1}}} \geq 0$.
By~\cref{prop_appen:local-feasible-option-with-hatct-one-step-globally-feasible}, it is one-step globally feasible.
Since this is true for $\ep$, \algname\ is globally feasible.
\end{proof} \label{sec:proofs}
\subsection{Domains}

\begin{figure}[h]
\centering
\includegraphics[width=\columnwidth]{figs/roomba.png}
\caption{In the Roomba CPOMDP environments, the robot must localize its belief (blue) before navigating to the goal region (green) while avoiding the penalty region (red line) and constrained regions (red box).}
\label{fig:roomba}
\end{figure}
